# Supplementary material for: Tuning nonradiative lifetimes via molecular aggregation
Source: arXiv:1611.09115 source file (2016-11-28)
Supplement: Supplementary file 1 [file sup_mat.pdf]

# Supplemental Material for: Tuning the nonradiative lifetime via molecular aggregation

A. Celestino[1] and A. Eisfeld[1]
[1]*Max Planck Institute for the Physics of Complex Systems, Nöthnitzer Strasse 38, 01187 Dresden, Germany*
(Dated: November 25, 2016)

In this Supplemental Material we provide details on the monomer and dimer models used to generate Letter's Fig. 1 (d) and Fig. 3.

## I. MONOMER MODEL AND ITS EQUATIONS OF MOTION

As discussed in the Letter, our monomer is a molecule interacting with an environment. Only a single electronically excited state $|\,\mathrm{e}\,\rangle$ is taken into account, together with the electronic ground state $|\,\mathrm{g}\,\rangle$. The electronic motion is coupled to internal and external vibrations in both ground and excited states. Using the framework of open quantum systems, we write the total Hamiltonian as

$$H_{\mathrm{tot}}^{(\mathrm{m})} = H_{\mathrm{sys}}^{(\mathrm{m})} + H_{\mathrm{bath}}^{(\mathrm{m})} + H_{\mathrm{int}}^{(\mathrm{m})}, \tag{1}$$

i.e. a sum of the "system" part $H_{\mathrm{sys}}^{(\mathrm{m})}$, the "bath" $H_{\mathrm{bath}}^{(\mathrm{m})}$, and the interaction between system and bath $H_{\mathrm{int}}^{(\mathrm{m})}$. The superscript (m) stands for "monomer" and was introduced to differentiate these symbols from their "dimer" counterparts, which will appear in Sec. (II). We include only a single normal mode coordinate [1] $q$ in the system degrees of freedom, which we call the "reaction coordinate". The potential energy surface associated to the reaction coordinate is assumed to be harmonic, with the same frequency $\omega$ in both electronic states. We further assume that the potential energy surfaces are shifted with respect to each other in energy, by the electronic transition energy $E_{\mathrm{e}}$, and in the reaction coordinate, by $q_{\mathrm{s}}$. The resulting potential energy surfaces are respectively $V_{\mathrm{g}}(q) = \omega^2 q^2/2$ for the electronic ground state and $V_{\mathrm{e}}(q) = \omega^2 (q - q_{\mathrm{s}})^2/2 + E_{\mathrm{e}}$ for the electronically excited state. This model of shifted harmonic potential energy surfaces for the modes implicitly incorporated in the system part is often used in the literature (see e.g. [2–5]) and was found to be reasonable in many cases (see e.g. [6, 7]). We consider a nonradiative decay channel to couple the electronically excited state either to the electronic ground state g or to a third electronic dark state d. The basic assumption is that no population flows from g (or d) back to e. For simplicity, we model this nonradiative decay channel as an imaginary potential [8] $-i\Gamma(q)|\,e\,\rangle\langle\,e\,| = -i\lambda\delta\left(q - q_{\mathrm{nr}}\right)|\,e\,\rangle\langle\,e\,|$, where $\lambda$ is the nonradiative decay strength and $q_{\mathrm{nr}}$ is the position of the nonradiative decay channel. The resulting non-Hermitian system Hamiltonian is

$$H_{\mathrm{sys}}^{(\mathrm{m})}(p, q) = H_{\mathrm{g}}(p, q)\,|\,\mathrm{g}\,\rangle\langle\,\mathrm{g}\,| + \left(H_{\mathrm{e}}(p, q) - i\Gamma(p, q)\right)|\,e\,\rangle\langle\,e\,|, \tag{2}$$

where $p$ is the kinetic energy operator (the commutator $[q, p] = i\hbar$). Introducing the bosonic creation operator for the ground and excited state potential energy surfaces, respectively $a_{\mathrm{g}}^{\dagger} = \sqrt{\omega/2\hbar}\,(q - ip/\omega)$ and $a_{\mathrm{e}} = a_{\mathrm{g}} - q_{\mathrm{s}}\sqrt{\omega/2\hbar}$ [3], the nuclear Hamiltonians $H_{\mathrm{g}}$ and $H_{\mathrm{e}}$ are

$$H_{\mathrm{g}}\left(a_{\mathrm{g}}, a_{\mathrm{g}}^{\dagger}\right) = \hbar\omega a_{\mathrm{g}}^{\dagger} a_{\mathrm{g}}, \tag{3}$$

$$H_{\mathrm{e}}\left(a_{\mathrm{e}}, a_{\mathrm{e}}^{\dagger}\right) = E_{\mathrm{e}} + \hbar\omega a_{\mathrm{e}}^{\dagger} a_{\mathrm{e}}. \tag{4}$$

The bath is a set of harmonic normal modes with frequencies $\omega_\lambda$ and creation (annihilation) operators $b_\lambda^{\dagger}$ ($b_\lambda$). This leads to the bath Hamiltonian

$$H_{\mathrm{bath}}^{(\mathrm{m})}(\{b_\lambda\}) = \sum_\lambda \hbar\omega_\lambda b_\lambda^{\dagger} b_\lambda. \tag{5}$$

We consider that the bath is linearly coupled to the system degrees of freedom [1, 2, 9]. As for the system coupling operator (to the bath) we use a model analogous to the one described in [3], with a slightly different system coupling operator

$$L_{\mathrm{sys}}^{(\mathrm{m})} = \left(a_{\mathrm{g}}^{\dagger} + a_{\mathrm{g}}\right)|\,\mathrm{g}\,\rangle\langle\,\mathrm{g}\,| + \left(a_{\mathrm{e}}^{\dagger} + a_{\mathrm{e}}\right)|\,\mathrm{e}\,\rangle\langle\,\mathrm{e}\,|. \tag{6}$$

Note that we couple the system to the bath through the dimensionless reaction coordinate $\sqrt{2\omega/\hbar}q = \left(a_{\mathrm{g}}^{\dagger} + a_{\mathrm{g}}\right)$ in the electronic ground state and to the shifted dimensionless reaction coordinate $\sqrt{2\omega/\hbar}\,(q - q_{\mathrm{s}}) = \left(a_{\mathrm{e}}^{\dagger} + a_{\mathrm{e}}\right)$ in the

electronic excited state. Later on, when we consider a quantum master equation for the system part, this system coupling operator will lead to vibrational relaxation towards the ground state of (i) $V_{\rm g}(q)$ in $|\,{\rm g}\,\rangle$ and (ii) $V_{\rm e}(q)$ in $|\,{\rm e}\,\rangle$. Our bath coupling operator is the sum of all bath normal mode coordinates [1]. The system-bath interaction Hamiltonian is given by

$$H_{\rm int}^{\rm (m)} = \left(a_{\rm g} + a_{\rm g}^\dagger - \sqrt{\frac{2\omega}{\hbar}}q_{\rm s}|\,{\rm e}\,\rangle\langle\,{\rm e}\,|\right)\sum_\lambda \kappa_\lambda\left(b_\lambda + b_\lambda^\dagger\right). \tag{7}$$

The weight of the bath coupling to a specific frequency $\tilde{\omega}$ is encoded in the bath spectral density $j\left(\tilde{\omega}\right) = \sum_\lambda \kappa_\lambda^2\delta(\tilde{\omega} - \omega_\lambda)$. We have chosen an Ohmic spectral density

$$j\left(\tilde{\omega}\right) = \theta\left(\tilde{\omega}\right)\gamma\tilde{\omega}e^{-\tilde{\omega}/\omega_0}, \tag{8}$$

where $\gamma$ and $\omega_0$ are real parameters, and the step function $\theta(\tilde{\omega})$ guarantees that we just consider positive frequencies. For all simulations shown in the Letter, we have fixed $\gamma = \hbar^2/\pi$ and the cutoff frequency $\omega_0 = 10\omega/\pi$.

Now we aim at obtaining an approximate equation of motion for the "system" alone, which includes only the degrees of freedom of $H_{\rm sys}^{\rm (m)}$. Our procedure follows [1]. We start from the equation of motion for the density operator of the complete system, formed by the system and bath degrees of freedom,

$$\frac{\partial\rho_{\rm tot}^{\rm (m)}(t)}{\partial t} = -\frac{i}{\hbar}\left[H_{\rm tot}^{\rm (m)}\rho_{\rm tot}^{\rm (m)}(t) - \rho_{\rm tot}^{\rm (m)}(t)\left(H_{\rm tot}^{\rm (m)}\right)^\dagger\right]. \tag{9}$$

Next, we trace out the bath degrees of freedom, i.e. those which are included in $H_{\rm bath}^{\rm (m)}$. This yields the reduced density operator (system density operator)

$$\rho_{\rm sys}^{\rm (m)} = {\rm Tr}_{\rm bath}\left\{\rho_{\rm tot}^{\rm (m)}\right\} = \sum_\lambda\sum_{n_\lambda}\langle\, n_\lambda\,|\rho_{\rm tot}^{\rm (m)}|\, n_\lambda\,\rangle, \tag{10}$$

in which we used the bath eigenbasis $\{|\,n_\lambda\,\rangle\}$ to represent the trace over bath degrees of freedom. Then we perform the Born and Markov approximations, obtaining a multilevel Redfield equation of motion in the energy representation. For simplicity, we perform the secular approximation and neglect pure dephasing [1], obtaining the following equation of motion:

$$\frac{\partial\rho_{\rm sys}^{\rm (m)}}{\partial t} = -\frac{i}{\hbar}\left[H_{\rm sys}^{\rm (m)}\rho_{\rm sys}^{\rm (m)} - \rho_{\rm sys}^{\rm (m)}\left(H_{\rm sys}^{\rm (m)}\right)^\dagger\right] + \mathcal{L}\left[\rho_{\rm sys}^{\rm (m)}\right]. \tag{11}$$

$\mathcal{L}$ is a dissipator, which can be written in the following Lindblad form

$$\mathcal{L}\left[\rho_{\rm sys}^{\rm (m)}\right] = \sum_{a,b}\left[A_{a,b}\rho_{\rm sys}^{\rm (m)}A_{a,b}^\dagger - \frac{1}{2}\left(A_{a,b}^\dagger A_{a,b}\rho_{\rm sys}^{\rm (m)} + \rho_{\rm sys}^{\rm (m)}A_{a,b}^\dagger A_{a,b}\right)\right], \tag{12}$$

where we have introduced the eigenbasis $\{|\,a\,\rangle\}$ of the Hermitian part of $H_{\rm sys}^{\rm (m)}$,

$$\frac{1}{2}\left[H_{\rm sys}^{\rm (m)} + \left(H_{\rm sys}^{\rm (m)}\right)^\dagger\right]|\,a\,\rangle = \epsilon_a^{\rm (m)}|\,a\,\rangle, \tag{13}$$

with the correspondent eigenspectrum $\left\{\epsilon_a^{\rm (m)}\right\}$, and the double sum in Eq. (12) runs over all eigenstates. The Lindblad operators $A_{a,b}$ are given by $A_{a,b} = \sqrt{k_{a\to b}}|\,b\,\rangle\langle\,a\,|$, with the transition rates

$$k_{a\to b} = C\left(\omega_{ab}\right)\left|\langle\,a\,|L_{\rm sys}^{\rm (m)}|\,b\,\rangle\right|^2, \tag{14}$$

where $\omega_{ab} = \left(\epsilon_a^{\rm (m)} - \epsilon_b^{\rm (m)}\right)/\hbar$ and

$$C\left(\omega_{ab}\right) = \frac{2\pi}{\hbar^2}\left(1 + n\left(\omega_{ab}\right)\right)\left(j\left(\omega_{ab}\right) - j\left(-\omega_{ab}\right)\right), \tag{15}$$

where

$$n\left(\omega_{ab}\right)=\frac{1}{e^{\hbar\omega_{ab}/k_{\mathrm{B}}T}-1} \tag{16}$$

is the Bose-Einstein distribution. Since we set $T=0$, $n\left(\omega_{ab}\right)=0$ for $\omega_{ab}>0$. Using the relation $1+n\left(\omega_{ab}\right)=-n\left(-\omega_{ab}\right)$ and Eq. (8) one can rewrite $C\left(\omega_{ab}\right)$ as

$$C\left(\omega_{ab}\right)=\frac{2\pi}{\hbar^{2}}\gamma\omega_{ab}e^{-\omega_{ab}/\omega_{0}},\ \omega_{ab}>0, \tag{17}$$

$$C\left(\omega_{ab}\right)=0,\ \omega_{ab}<0. \tag{18}$$

Note that setting pure dephasing to zero implies $C(0)=0$ [1].

## II. DIMER MODEL AND ITS EQUATIONS OF MOTION

We discussed in the Letter a transition-dipole-dipole-interacting dimer composed of two identical monomers (for details on the monomer model see Sec. (I)) at fixed orientation and distance between their centers of mass. As one can see from the Letter's Eq. (1), we take into account just resonance coupling between $|\,\pi_1\,\rangle=|\,\mathrm{e}\,\rangle|\,\mathrm{g}\,\rangle$ and $|\,\pi_2\,\rangle=|\,\mathrm{g}\,\rangle|\,\mathrm{e}\,\rangle$ electronic states. We assume that the electronic dipole-dipole coupling matrix element is independent of nuclear coordinates [10]. We further assume that the monomers and their respective environments are formed by disjoint sets of degrees of freedom. The bath spectral densities are the same for the both baths (please see Sec. (I)). The resulting total Hamiltonian is given by

$$H_{\mathrm{tot}}^{(\mathrm{d})}=H_{\mathrm{tot}}^{(\mathrm{m1})}+H_{\mathrm{tot}}^{(\mathrm{m2})}+J\left(|\,\pi_1\,\rangle\langle\,\pi_2\,|+|\,\pi_2\,\rangle\langle\,\pi_1\,|\right), \tag{19}$$

where the parameter $J$ is the transition dipole-dipole interaction strength and "m1" refers to "monomer 1" while "m2" refers to "monomer 2". Note that the electronic states $|\,\mathrm{gg}\,\rangle=|\,\mathrm{g}\,\rangle|\,\mathrm{g}\,\rangle$ and $|\,\mathrm{ee}\,\rangle=|\,\mathrm{e}\,\rangle|\,\mathrm{e}\,\rangle$ do not couple to the single excitation manifold $\{|\,\pi_1\,\rangle,|\,\pi_2\,\rangle\}$ and therefore we no longer take these electronic states into account.

Using the framework of open quantum systems, we can separate the total Hamiltonian $H_{\mathrm{tot}}^{(\mathrm{d})}$ into a system part $H_{\mathrm{sys}}^{(\mathrm{d})}$, a bath part $H_{\mathrm{bath}}^{(\mathrm{d})}$ and a system-bath interaction $H_{\mathrm{int}}^{(\mathrm{d})}$. The system Hamiltonian is

$$H_{\mathrm{sys}}^{(\mathrm{d})}=H_{\mathrm{sys}}^{(\mathrm{m1})}+H_{\mathrm{sys}}^{(\mathrm{m2})}+J\left(|\,\pi_1\,\rangle\langle\,\pi_2\,|+|\,\pi_2\,\rangle\langle\,\pi_1\,|\right)=H_{\mathrm{ex}}, \tag{20}$$

where $H_{\mathrm{ex}}$ is defined in Eq. (1) of the Letter. The dimer bath Hamiltonian is given by $H_{\mathrm{bath}}^{(\mathrm{d})}=H_{\mathrm{bath}}^{(\mathrm{m1})}+H_{\mathrm{bath}}^{(\mathrm{m2})}$ while the dimer system-bath interaction is given by $H_{\mathrm{int}}^{(\mathrm{d})}=H_{\mathrm{int}}^{(\mathrm{m1})}+H_{\mathrm{int}}^{(\mathrm{m2})}$.

As in Sec. (I), we aim at obtaining an approximate equation of motion for the dimer's system part alone, which includes only the degrees of freedom of $H_{\mathrm{ex}}$. We follow the same procedure as described in Sec. (I) and [1], obtaining the following multilevel Redfield equation for the dimer's system density operator $\rho_{\mathrm{sys}}^{(\mathrm{d})}$:

$$\frac{\partial\rho_{\mathrm{sys}}^{(\mathrm{d})}}{\partial t}=-\frac{i}{\hbar}\left[H_{\mathrm{sys}}^{(\mathrm{d})}\rho_{\mathrm{sys}}^{(\mathrm{d})}-\rho_{\mathrm{sys}}^{(\mathrm{d})}\left(H_{\mathrm{sys}}^{(\mathrm{d})}\right)^{\dagger}\right]+\mathcal{L}_1\left[\rho_{\mathrm{sys}}^{(\mathrm{d})}\right]+\mathcal{L}_2\left[\rho_{\mathrm{sys}}^{(\mathrm{d})}\right], \tag{21}$$

with

$$\begin{aligned}\mathcal{L}_j\left[\rho_{\mathrm{sys}}^{(\mathrm{d})}\right]=\sum_{\alpha,\beta}\Bigg\{&A_{\alpha,\beta}^{(\mathrm{m}j)}\rho_{\mathrm{sys}}^{(\mathrm{d})}\left(A_{\alpha,\beta}^{(\mathrm{m}j)}\right)^{\dagger}\\&-\frac{1}{2}\left[\left(A_{\alpha,\beta}^{(\mathrm{m}j)}\right)^{\dagger}A_{\alpha,\beta}^{(\mathrm{m}j)}\rho_{\mathrm{sys}}^{(\mathrm{d})}+\rho_{\mathrm{sys}}^{(\mathrm{d})}\left(A_{\alpha,\beta}^{(\mathrm{m}j)}\right)^{\dagger}A_{\alpha,\beta}^{(\mathrm{m}j)}\right]\Bigg\}.\end{aligned} \tag{22}$$

In Eq. (22) we have introduced the eigenbasis $\{|\,\alpha\,\rangle\}$ of the Hermitian part of $H_{\mathrm{sys}}^{(\mathrm{d})}$,

$$\frac{1}{2}\left[H_{\mathrm{sys}}^{(\mathrm{d})}+\left(H_{\mathrm{sys}}^{(\mathrm{d})}\right)^{\dagger}\right]|\,a\,\rangle=\epsilon_{\alpha}^{(\mathrm{d})}|\,\alpha\,\rangle, \tag{23}$$

with the correspondent eigenspectrum $\left\{\epsilon_\alpha^{(\mathrm{d})}\right\}$, and the double sum in Eq. (22) runs over all eigenstates. The Lindblad operator $A_{\alpha,\beta}^{(\mathrm{m}j)} = \sqrt{k_{\alpha\to\beta}^{(\mathrm{m}j)}}|\,\beta\,\rangle\langle\,\alpha\,|$ and the transition rates are given by

$$k_{\alpha\to\beta}^{(\mathrm{m}j)} = C\left(\omega_{\alpha\beta}\right)\left|\langle\,\alpha\,|L_{\mathrm{sys}}^{(\mathrm{m}j)}|\,\beta\,\rangle\right|^2 , \tag{24}$$

where $\omega_{\alpha\beta} = \left(\epsilon_\alpha^{(\mathrm{d})} - \epsilon_\beta^{(\mathrm{d})}\right)/\hbar$ and $C\left(\omega_{\alpha\beta}\right)$ was already defined in Eqs. (15), (17), and (18), where one needs to replace $\omega_{ab}$ by $\omega_{\alpha\beta}$.

---


[1] V. May and O. Kühn; *Charge and energy transfer dynamics in molecular systems*; John Wiley & Sons (2011).
[2] S. Mukamel; *Nonlinear Optical Spectroscopy*; Oxford University Press (1995).
[3] J. Roden, W. T. Strunz, K. B. Whaley and A. Eisfeld; The Journal of Chemical Physics **137** 204110 (2012).
[4] B. Wolfseder and W. Domcke; Chemical Physics Letters **235** 370 (1995).
[5] D. Egorova, M. F. Gelin, M. Thoss, H. Wang and W. Domcke; The Journal of Chemical Physics **129** 214303 (2008).
[6] J. Roden, A. Eisfeld, M. Dvok, O. Bnermann and F. Stienkemeier; The Journal of Chemical Physics **134** 054907 (2011).
[7] A. Ishizaki, T. R. Calhoun, G. S. Schlau-Cohen and G. R. Fleming; Phys. Chem. Chem. Phys. **12** 7319 (2010).
[8] F. Gemperle, F. Gadea and P. Durand; Chemical Physics Letters **291** 517 (1998).
[9] U. Weiss; *Quantum Dissipative Systems*; World Scientific, Singapore (2008).
[10] A. Witkowski and W. Moffitt; The Journal of Chemical Physics **33** 872 (1960).
